# Supplementary material for: Electromyogram (EMG) Removal by Adding Sources of EMG (ERASE) -- A novel ICA-based algorithm for removing myoelectric artifacts from EEG -- Part 2
Source: arXiv:2007.03136 source file (2020-07-07)
Supplement: Supplementary file 1 [file Appendix_part2.pdf]

## Part 2. Supplementary results

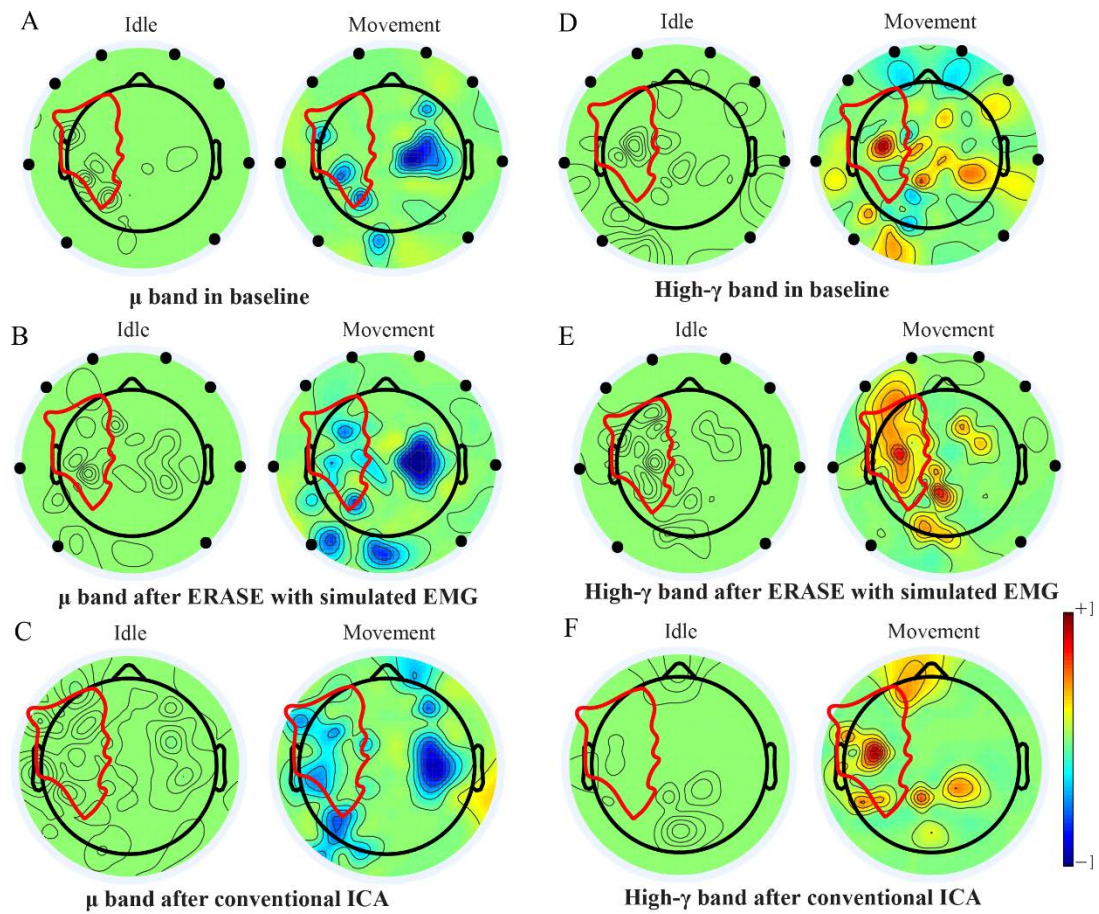

Fig. 1. Brain topography maps of z-scored  $\mu$  and high- $\gamma$  power before and after artifact rejection with ERASE with simulated EMG and conventional ICA on the Subject 2. Time for idle is 1 second before movement. Time for movement is 2 seconds. Only electrodes whose z-scored power of  $\mu$  and high- $\gamma$  during idle time and movement was significantly different were shown (Wilcoxon rank sum test). P-value for significant difference was 0.05. The black dots outlined the position of the added virtual electrodes. The red outline in each subfigure denoted the HAs.

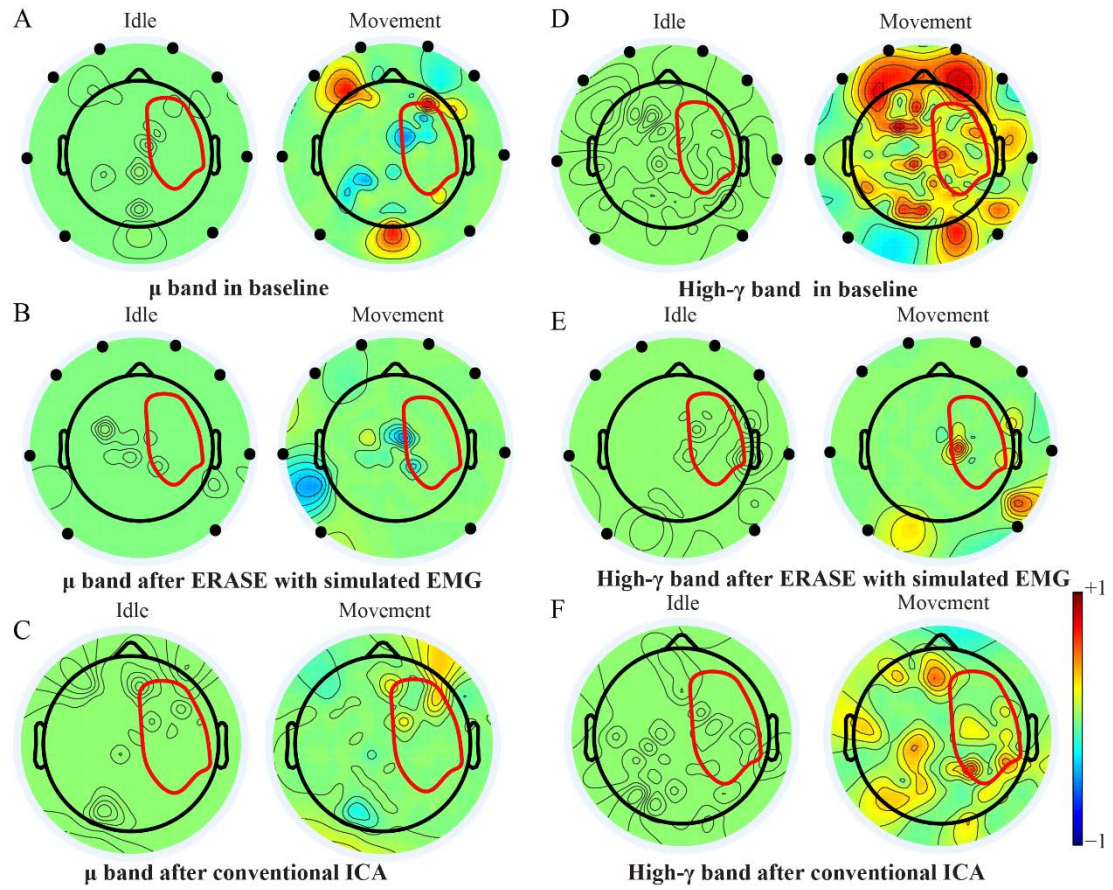

Fig. 2. Brain topography maps of z-scored  $\mu$  and high- $\gamma$  power before and after artifact rejection with ERASE with simulated EMG and conventional ICA on the Subject 3. Time for idle is 1 second before movement. Time for movement is 2 seconds. Only electrodes whose z-scored power of  $\mu$  and high- $\gamma$  during idle time and movement was significantly different were shown (Wilcoxon rank sum test). P-value for significant difference was 0.05. The black dots outlined the position of the added virtual electrodes. The red outline in each subfigure denoted the HAs.

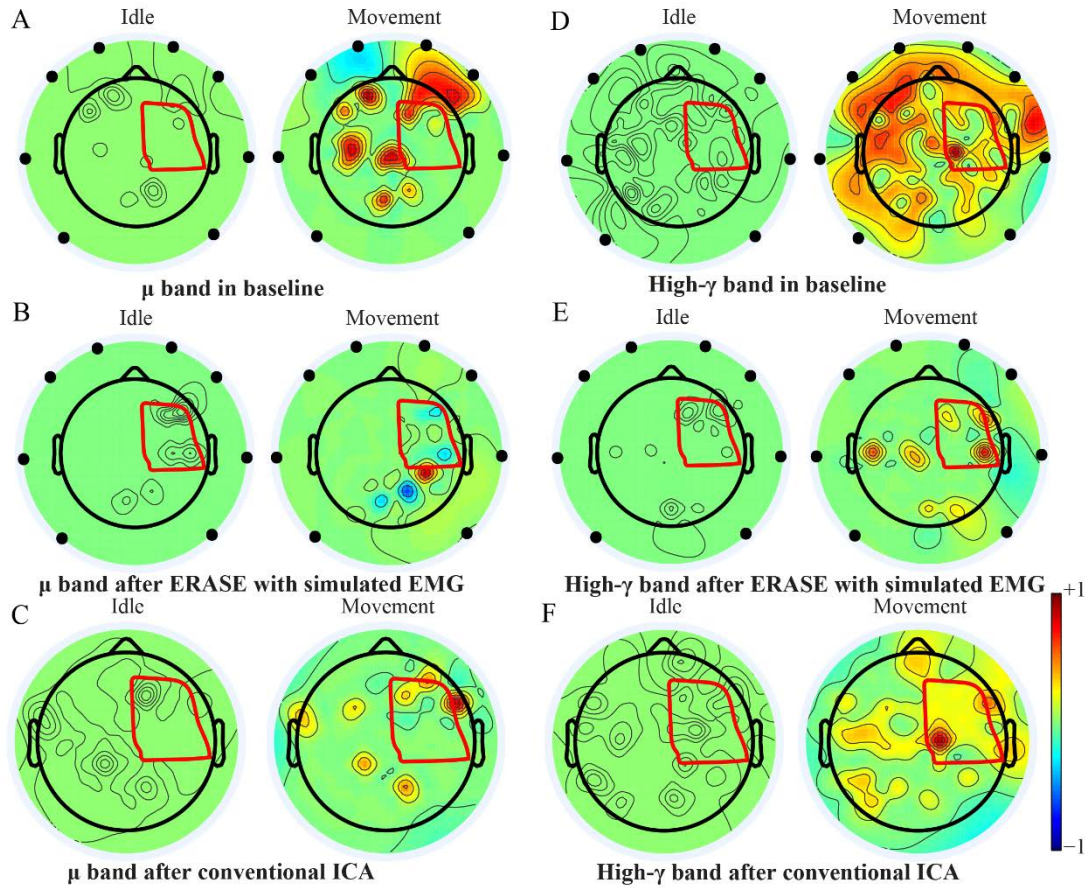

Fig. 3. Brain topography maps of z-scored  $\mu$  and high- $\gamma$  power before and after artifact rejection with ERASE with simulated EMG and conventional ICA on the Subject 4. Time for idle is 1 second before movement. Time for movement is 2 seconds. Only electrodes whose z-scored power of  $\mu$  and high- $\gamma$  during idle time and movement was significantly different were shown (Wilcoxon rank sum test). P-value for significant difference was 0.05. The black dots outlined the position of the added virtual electrodes. The red outline in each subfigure denoted the HAs.



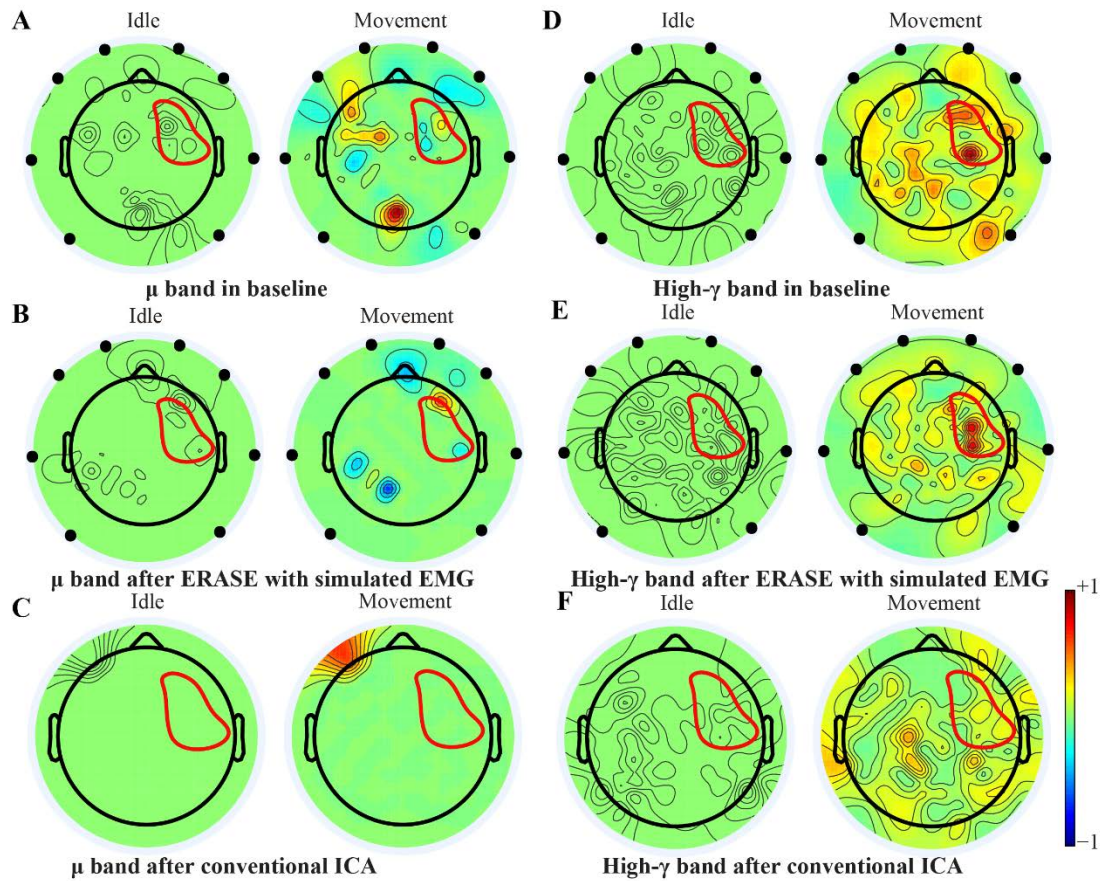

Fig. 4. Brain topography maps of z-scored  $\mu$  and high- $\gamma$  power before and after artifact rejection with ERASE with simulated EMG and conventional ICA on the Subject 5. Time for idle is 1 second before movement. Time for movement is 2 seconds. Only electrodes whose z-scored power of  $\mu$  and high- $\gamma$  during idle time and movement was significantly different were shown (Wilcoxon rank sum test). P-value for significant difference was 0.05. The black dots outlined the position of the added virtual electrodes. The red outline in each subfigure denoted the HAS.

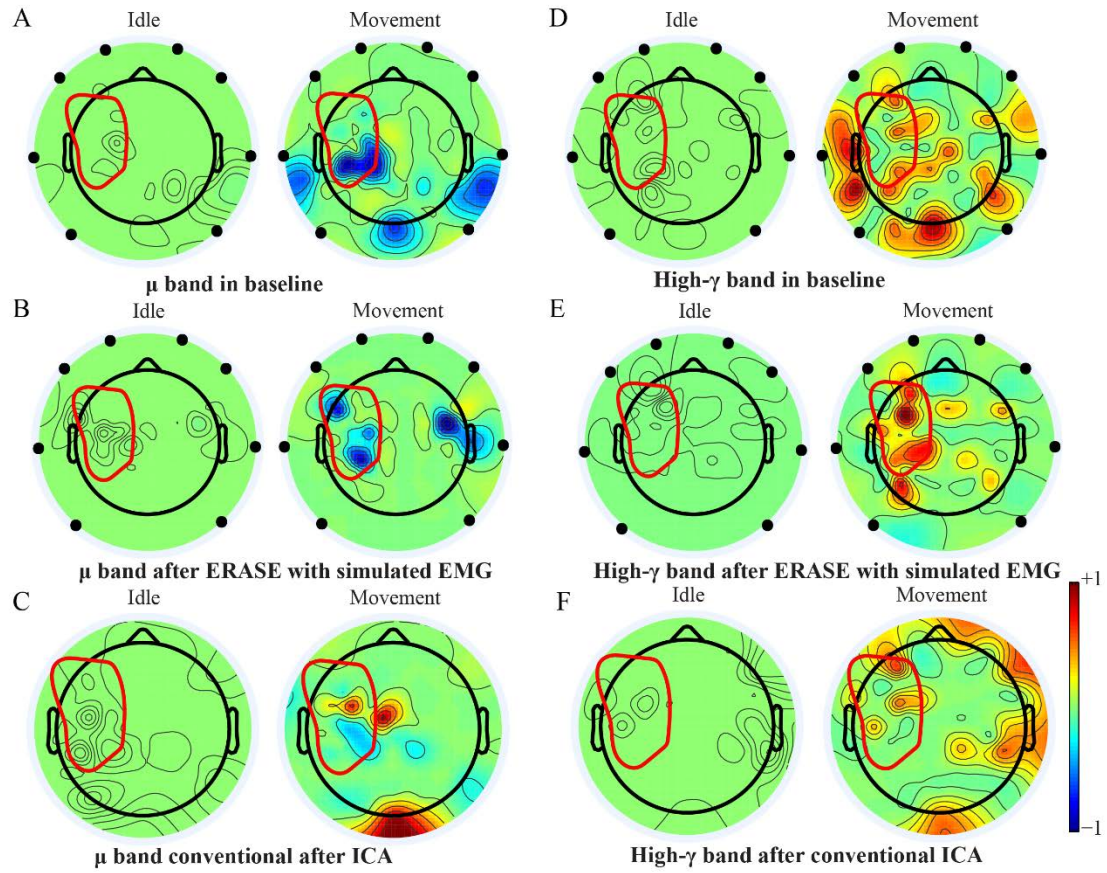

Fig. 5. Brain topography maps of z-scored  $\mu$  and high- $\gamma$  power before and after artifact rejection with ERASE with simulated EMG and conventional ICA on the Subject 6. Time for idle is 1 second before movement. Time for movement is 2 seconds. Only electrodes whose z-scored power of  $\mu$  and high- $\gamma$  during idle time and movement was significantly different were shown (Wilcoxon rank sum test). P-value for significant difference was 0.05. The black dots outlined the position of the added virtual electrodes. The red outline in each subfigure denoted the HAs.

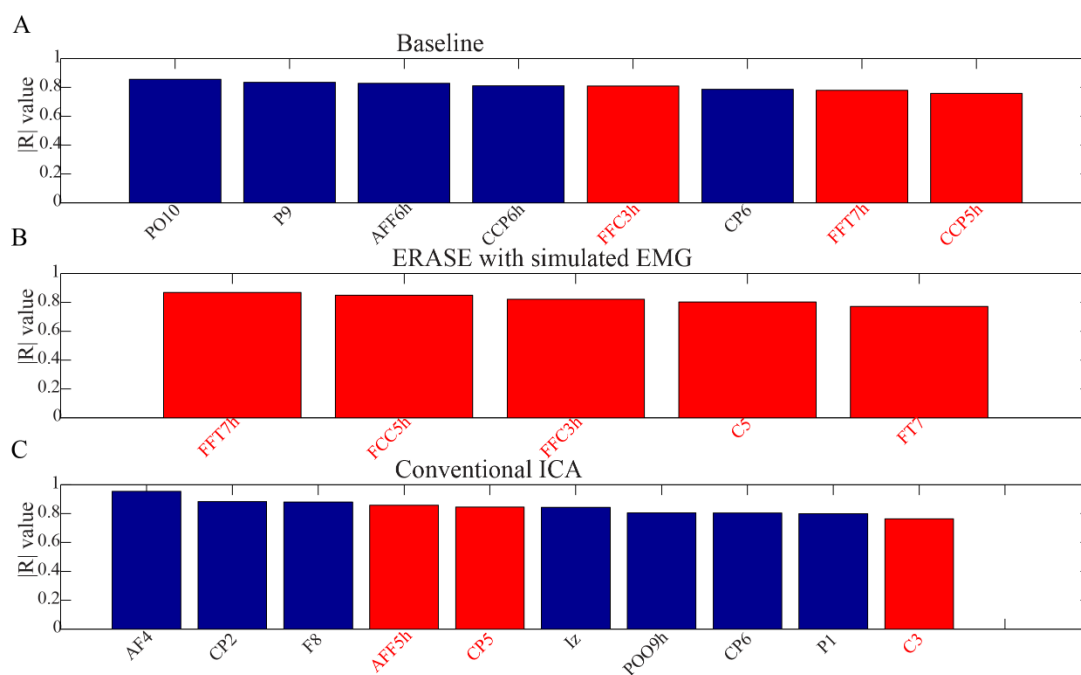

Fig. 6. Bar graphs for showing the electrodes with significant correlation in three conditions (baseline, after ERASE with simulated EMG and after conventional ICA). Here, the correlation coefficients were absolute values from 0 to 1. Data were from Subject 2. Blue bars denoted the electrodes with significant correlation in the NHAs, and red bars were the ones in HAs. A. the electrodes with significant correlation before ERASE. B. the electrodes with significant correlation after ERASE with simulated EMG. C. the electrodes with significant correlation after conventional ICA.

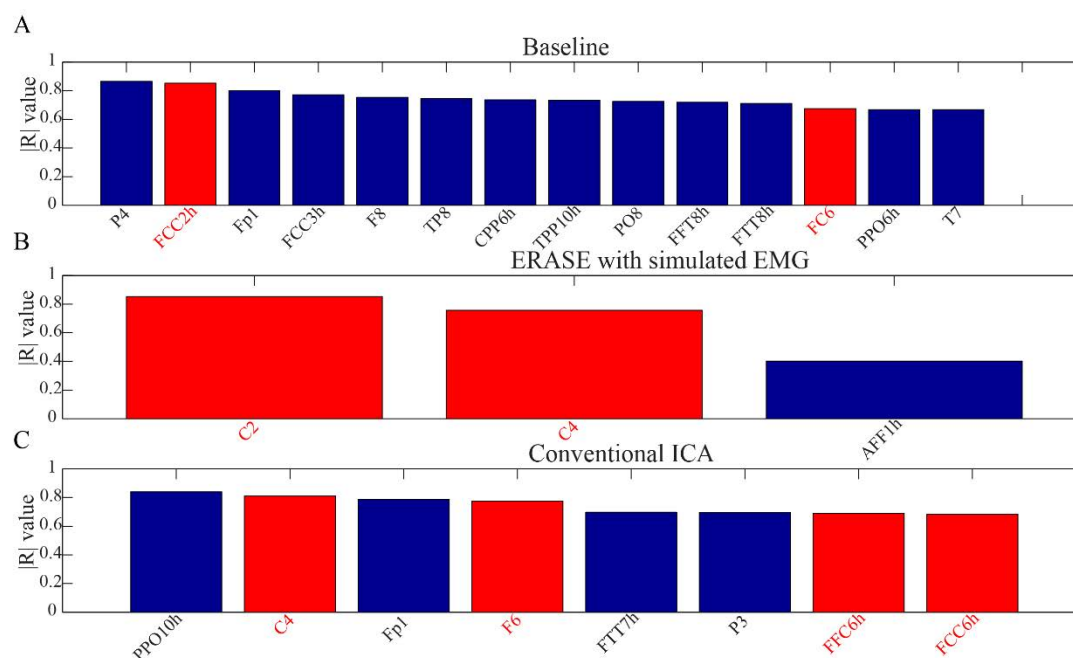

Fig. 7. Bar graphs for showing the electrodes with significant correlation in three conditions (baseline, after ERASE with simulated EMG and after conventional ICA). Here, the correlation coefficients were absolute values from 0 to 1. Data were from Subject 3. Blue bars denoted the electrodes with significant correlation in the NHAs, and red bars were the ones in HAs. A. the

electrodes with significant correlation before ERASE. B. the electrodes with significant correlation after ERASE with simulated EMG. C. the electrodes with significant correlation after conventional ICA.

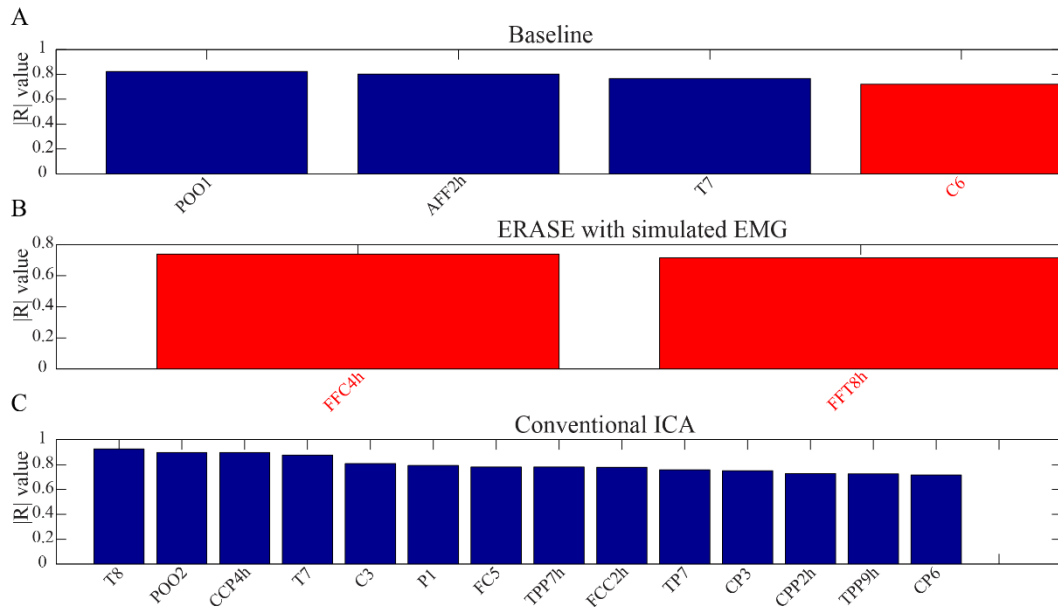

Fig. 8. Bar graphs for showing the electrodes with significant correlation in three conditions (baseline, after ERASE with simulated EMG and after conventional ICA). Here, the correlation coefficients were absolute values from 0 to 1. Data were from Subject 4. Blue bars denoted the electrodes with significant correlation in the NHAs, and red bars were the ones in HAs. A. the electrodes with significant correlation before ERASE. B. the electrodes with significant correlation after ERASE with simulated EMG. C. the electrodes with significant correlation after conventional ICA.

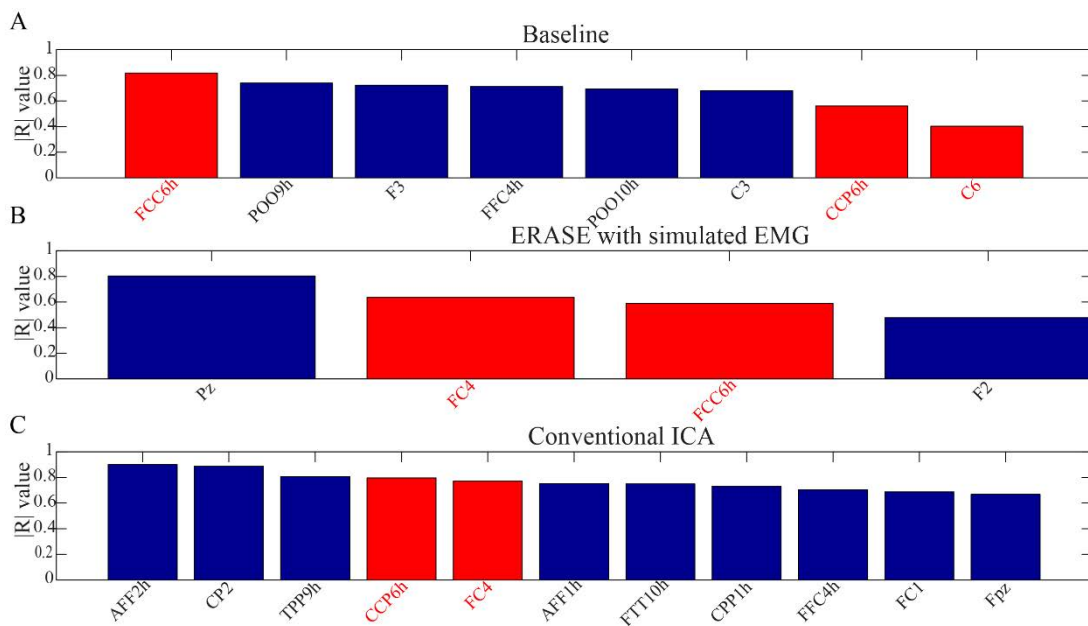

Fig. 9. Bar graphs for showing the electrodes with significant correlation in three conditions (baseline, after ERASE with simulated EMG and after conventional ICA). Here, the correlation coefficients were absolute values from 0 to 1. Data were from Subject 5. Blue bars denoted the

electrodes with significant correlation in the NHAs, and red bars were the ones in HAs. A. the electrodes with significant correlation before ERASE. B. the electrodes with significant correlation after ERASE with simulated EMG. C. the electrodes with significant correlation after conventional ICA.

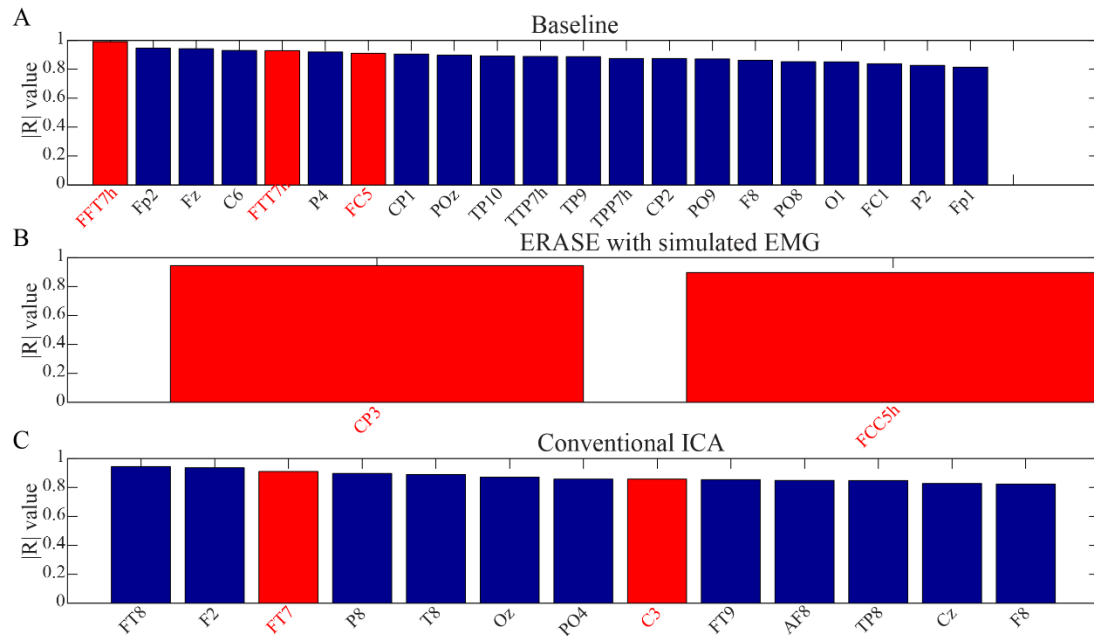

Fig. 10. Bar graphs for showing the electrodes with significant correlation in three conditions (baseline, after ERASE with simulated EMG and after conventional ICA). Here, the correlation coefficients were absolute values from 0 to 1. Data were from Subject 6. Blue bars denoted the electrodes with significant correlation in the NHAs, and red bars were the ones in HAs. A. the electrodes with significant correlation before ERASE. B. the electrodes with significant correlation after ERASE with simulated EMG. C. the electrodes with significant correlation after conventional ICA.



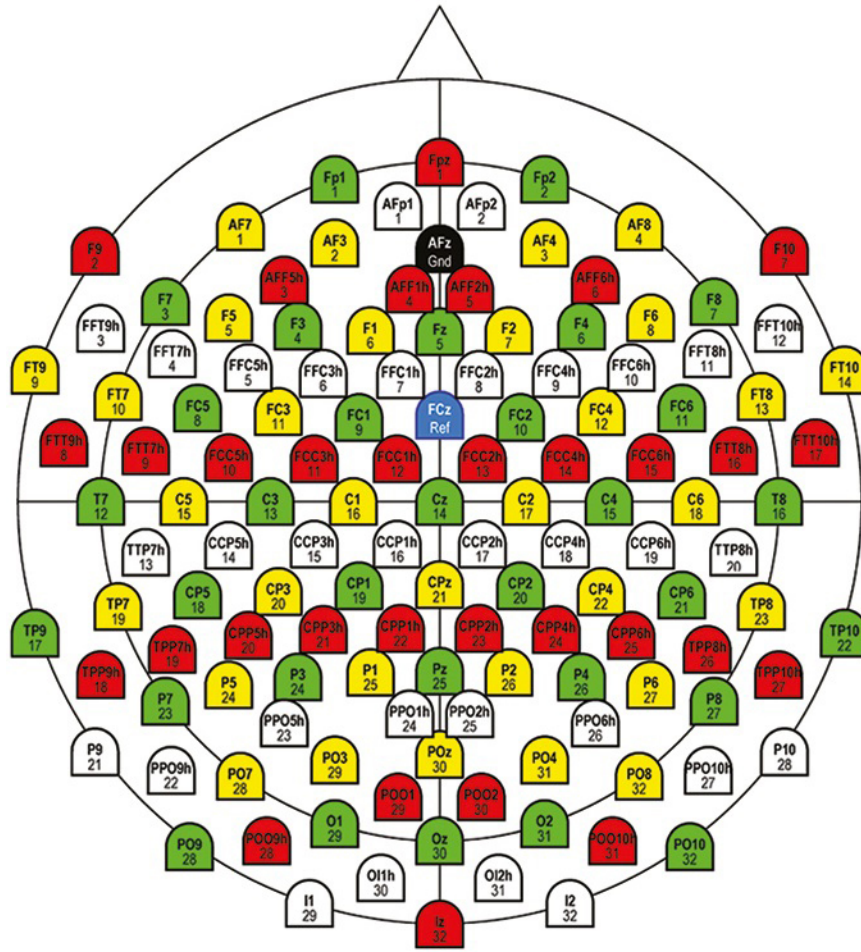

Fig. 11. The 2D image of the electrode locations for the ActiCap EEG cap (Brain Products).
